# Supplementary material for: BlockDrop: Dynamic Inference Paths in Residual Networks
Source: arXiv:1711.08393 source file (2019-01-28)
Supplement: Supplementary file 1 [file supplement.tex]

\begin{table}[]
\centering
\begin{tabular}{llllll}
ImageNet   &                   & FLOPs                & Block Usage  & Accuracy & Speed-up \\
ResNet-50  & \system           & 8.18E+09 \pm 0.00E+00 & 16.0 \pm 0.0 & 75.3     & --       \\
           & \system \gamma=5  & ?                     & ?            & ?        & ?        \\
           &                   &                       &              &          &          \\
ResNet-101 & Original          & 1.56E+10 \pm 0.00E+00 & 33.0 \pm 0.0 & 76.4     & --       \\
           & \system \gamma=2  & 9.85E+09 \pm 3.34E+08 & 18.8 \pm 0.8 & 75.2     & 36.9\%   \\
           & \system \gamma=5  & 1.25E+10 \pm 4.26E+08 & 24.8 \pm 1.0 & 76.4     & 19.9\%   \\
           & \system \gamma=10 & 1.47E+10 \pm 4.02E+08 & 29.7 \pm 0.9 & 76.8     & 5.7\%    \\
           &                   &                       &              &          &          \\
CIFAR-10   &                   &                       &              &          &          \\
ResNet-32  & Original          & 1.38E+08 \pm 0.00E+00 & 15.0 \pm 0.0 & 92.3     & --       \\
           & \system \gamma=5  & 8.66E+07 \pm 1.40E+07 & 6.9 \pm 1.6  & 91.3     & 37.2\%   \\
           &                   &                       &              &          &          \\
ResNet-110 & Original          & 5.06E+08 \pm 0.00E+00 & 56.0 \pm 0.0 & 93.2     & --       \\
           & \system \gamma=2  & 1.18E+08 \pm 2.46E+07 & 10.3 \pm 2.7 & 91.9     & 76.7\%   \\
           & \system \gamma=5  & 1.51E+08 \pm 3.24E+07 & 13.8 \pm 3.5 & 93.0     & 70.1\%   \\
           & \system \gamma=10 & 1.81E+08 \pm 3.43E+07 & 16.9 \pm 3.7 & 93.6     & 64.3\%   \\
           &                   &                       &              &          &          \\
CIFAR-100  &                   &                       &              &          &          \\
ResNet-32  & Original          & 1.38E+08 \pm 0.00E+00 & 15.0 \pm 0.0 & 67.2     & --       \\
           & \system \gamma=5  & 1.44E+08 \pm 1.02E+07 & 13.0 \pm 1.1 & 68.45    & -4.3\%   \\
           &                   &                       &              &          &          \\
ResNet-110 & Original          & 5.06E+08 \pm 0.00E+00 & 54.0 \pm 0.0 & 72.2     & --       \\
           & \system \gamma=5  & 3.06E+08 \pm 3.86E+06 & 30.2 \pm 0.4 & 73.7     & 39.5\%   \\

\end{tabular}
\caption{All results}
\label{table:all_results}
\end{table}
